# Supplementary material for: MBE-CASSCF Approach for the Accurate Treatment of Large Active Spaces
Source: arXiv:2403.17836 ancillary file (2024-06-18)
Supplement: Supplementary file 1 [file si.pdf]

# Supporting Information: An MBE-CASSCF Approach for the Accurate Treatment of Large Active Spaces


Jonas Greiner,†,§ Ivan Gianni,‡,§ Tommaso Nottoli,‡ Filippo Lipparini,*,‡ Janus J. Eriksen,*,¶ and Jürgen Gauss*,†

†*Department Chemie, Johannes Gutenberg-Universität Mainz Duesbergweg 10–14, 55128 Mainz, Germany*

‡*Dipartimento di Chimica e Chimica Industriale, Università di Pisa Via G. Moruzzi 13, Pisa, 56124, Italy*

¶*DTU Chemistry, Technical University of Denmark Kemitorvet Bldg. 206, 2800 Kgs. Lyngby, Denmark*

§*These authors contributed equally*

E-mail: filippo.lipparini@unipi.it; janus@dtu.dk; gauss@uni-mainz.de


The orbital indices are divided as follows: The indices $\{i, j, k, \ldots\}$, $\{u, v, w, \ldots\}$, and $\{a, b, c, \ldots\}$ describe the occupied, active, and virtual orbitals with respect to the CASSCF active space, respectively. The active space is further divided through the indices $\{i', j', k', \ldots\}$, $\{u', v', w', \ldots\}$, and $\{a', b', c', \ldots\}$, which describe the occupied, active, and virtual orbitals with respect to the increment active space within the CASSCF active space, respectively. Finally, the increment active is additionally divided through the indices $\{i'', j'', k'', \ldots\}$ and $\{a'', b'', c'', \ldots\}$, which describe the occupied and virtual orbitals of the reference determinant within the increment active space.

# MBEs of RDMs and Generalized Fock Matrices

The energy and orbital gradient constructed from many-body expanded RDMs will be different from the direct expansion of these quantities whenever the expansion space includes occupied orbitals and the expansion in question is truncated. The reason for this can be illustrated using a minimal example, in which the MBE energy is considered at expansion order 2 for a system with two occupied orbitals, $i$ and $j$, and one virtual orbital, $a$:

$$
\begin{aligned}
E^{(2)} &= \epsilon^{\text{corr}}_{i'a'} + \epsilon^{\text{corr}}_{j'a'} \\
&= (\mathbf{D}^{\text{corr}}_{i'a'})_{i'i'} \left(\mathbf{F}^{I}_{i'a'}\right)_{i'i'} + (\mathbf{D}^{\text{corr}}_{i'a'})_{i'a'} \left(\mathbf{F}^{I}_{i'a'}\right)_{i'a'} + (\mathbf{D}^{\text{corr}}_{i'a'})_{a'i'} \left(\mathbf{F}^{I}_{i'a'}\right)_{a'i'} \\
&\quad + (\mathbf{D}^{\text{corr}}_{i'a'})_{a'a'} \left(\mathbf{F}^{I}_{i'a'}\right)_{a'a'} + \left(\mathbf{D}^{\text{corr}}_{j'a'}\right)_{j'j'} \left(\mathbf{F}^{I}_{j'a'}\right)_{j'j'} + \left(\mathbf{D}^{\text{corr}}_{j'a'}\right)_{j'a'} \left(\mathbf{F}^{I}_{j'a'}\right)_{j'a'} \\
&\quad + \left(\mathbf{D}^{\text{corr}}_{j'a'}\right)_{a'j'} \left(\mathbf{F}^{I}_{j'a'}\right)_{a'j'} + \left(\mathbf{D}^{\text{corr}}_{j'a'}\right)_{a'a'} \left(\mathbf{F}^{I}_{j'a'}\right)_{a'a'} \\
&\quad + \text{two electron terms} \\
&= \sum_{k'b'} \left( (\mathbf{D}^{\text{corr}}_{i'a})_{k'b'} + \left(\mathbf{D}^{\text{corr}}_{j'a'}\right)_{k'b'} \right) h_{k'b'} \\
&\quad + \sum_{k'b'} (\mathbf{D}^{\text{corr}}_{i'a'})_{k'b'} \left(2(k'b'|j'j') - (k'j'|j'b')\right) + \sum_{k'b'} \left(\mathbf{D}^{\text{corr}}_{j'a}\right)_{k'b'} \left(2(k'b'|i'i') - (k'i'|i'b')\right) \\
&\quad + \text{two electron terms}
\end{aligned}
\tag{1}
$$

This second-order MBE energy cannot be divided into contributions from individual RDM increments unless the individual incremental 1-RDM is immediately contracted with the corresponding elements of the inactive Fock matrix. Therefore, the MBE energy from such an expansion cannot be reproduced from an MBE of the RDMs. The same arguments hold for the construction of the generalized Fock matrix in the determination of orbital gradients.

# Incremental Generalized Fock Matrix

The following elements contribute to an MBE of the generalized Fock matrix:

$$\begin{aligned}
\left(\mathbf{F}^{\text{corr}}_{u'}\right)_{ip} &= \left(\mathbf{F}_{u'}\right)_{ip} - \left(\mathbf{F}^{\text{ref}}_{u'}\right)_{ip} \\
&= 2\left(F^I_{pi} + \left(\mathbf{F}^A_{u'}\right)_{pi}\right) - 2\left(F^I_{pi} + \sum_{j''}\left(2(pi|j''j'') - (pj''|j''i)\right)\right) \\
&= 2\left(\sum_{v'w'}\left(\mathbf{D}_{u'}\right)_{v'w'}\left((pi|v'w') - \frac{1}{2}(pw'|v'i)\right) - \sum_{j''}\left(2(pi|j''j'')-)(pj''|j''i)\right)\right)
\end{aligned} \quad (2)$$

$$\begin{aligned}
\left(\mathbf{F}^{\text{corr}}_{u'}\right)_{i'p} &= \left(\mathbf{F}_{u'}\right)_{i'p} - \left(\mathbf{F}^{\text{ref}}_{u'}\right)_{i'p} \\
&= 2\left(F^I_{pi'} + \left(\mathbf{F}^A_{u'}\right)_{pi'}\right) - 2\left(F^I_{pi'} + \sum_{j''}\left(2(pi'|j''j'') - (pj''|j''i')\right)\right) \\
&= 2\left(\sum_{v'w'}\left(\mathbf{D}_{u'}\right)_{v'w'}\left((pi'|v'w') - \frac{1}{2}(pw'|v'i')\right) - \sum_{j''}\left(2(pi'|j''j'') - (pj''|j''i')\right)\right)
\end{aligned} \quad (3)$$

$$\begin{aligned}
\left(\mathbf{F}^{\text{corr}}_{u'}\right)_{i''p} &= \left(\mathbf{F}_{u'}\right)_{i''p} - \left(\mathbf{F}^{\text{ref}}_{u'}\right)_{i''p} \\
&= \sum_{v'}\left(\mathbf{D}_{u'}\right)_{i''v'} F^I_{pv'} + \sum_{v'w'x'}\left(\mathbf{d}_{u'}\right)_{i''v'w'x'}(pv'|w'x') \\
&\quad - \left(2F^I_{pi''} + \sum_{j''}\left(4(pi''|j''j'') - 2(pj''|j''i'')\right)\right)
\end{aligned} \quad (4)$$

$$\left(\mathbf{F}^{\text{corr}}_{u'}\right)_{a''p} = \left(\mathbf{F}_{u'}\right)_{a''p} - \left(\mathbf{F}^{\text{ref}}_{u'}\right)_{a''p} = \sum_{v'}\left(\mathbf{D}_{u'}\right)_{a''v'} F^I_{pv'} + \sum_{v'w'x'}\left(\mathbf{d}_{u'}\right)_{a''v'w'x'}(pv'|w'x') \quad (5)$$

$$\left(\mathbf{F}^{\text{corr}}_{u'}\right)_{a'p} = \left(\mathbf{F}_{u'}\right)_{a'p} - \left(\mathbf{F}^{\text{ref}}_{u'}\right)_{a'p} = 0 \quad (6)$$

All elements $\left(\mathbf{F}^{\text{corr}}_{u'}\right)_{i'p}$, $\left(\mathbf{F}^{\text{corr}}_{u'}\right)_{a'p}$, $\left(\mathbf{F}^{\text{corr}}_{u'}\right)_{i''p}$ and $\left(\mathbf{F}^{\text{corr}}_{u'}\right)_{a''p}$ will contribute to the active-general block of the correlated generalized Fock matrix, $F^{\text{corr}}_{up}$. The elements $\left(\mathbf{F}^{\text{corr}}_{u'}\right)_{ip}$ include contractions between the 1-RDM and the inactive Fock matrix and can therefore be constructed from an MBE of the 1-RDM. All incremental contributions to the generalized Fock matrix exclusively depend on the RDM elements of the increment active space.

# Active-Active Block of the Hessian Diagonal

The derivation of the active-active block of the Hessian diagonal starts from equations 21a and 21b in Ref. S1:

$$
\begin{aligned}
\frac{\partial E}{\partial \kappa_{uv} \partial \kappa_{uv}} &= \omega_{uvuv} - \omega_{vuuv} - \omega_{uvvu} + \omega_{vuvu} \\
&= \frac{\partial E}{\partial U_{uv} \partial U_{uv}} + \delta_{vu}(F_{uv} + F_{vu}) - \frac{\partial E}{\partial U_{vu} \partial U_{uv}} - \delta_{uu}(F_{vv} + F_{vv}) - \frac{\partial E}{\partial U_{uv} \partial U_{vu}} \\
&\quad - \delta_{vv}(F_{uu} + F_{uu}) + \frac{\partial E}{\partial U_{vu} \partial U_{vu}} + \delta_{uv}(F_{vu} + F_{uv}) \\
&= 2D_{uu}h_{vv} + 4\sum_{pq} \left(d_{uupq}(vv|pq) + \left(d_{uqpu} + d_{uqup}\right)(vp|vq)\right) \\
&\quad - 2D_{vu}h_{uv} - 4\sum_{pq} \left(d_{uvpq}(uv|pq) + \left(d_{uqpv} + d_{uqvp}\right)(up|vq)\right) \\
&\quad - 2D_{uv}h_{vu} - 4\sum_{pq} \left(d_{vupq}(vu|pq) + \left(d_{vqpu} + d_{vqup}\right)(vp|uq)\right) \\
&\quad + 2D_{vv}h_{uu} + 4\sum_{pq} \left(d_{vvpq}(uu|pq) + \left(d_{vqpv} + d_{vqvp}\right)(up|uq)\right) \\
&\quad + 2\delta_{uv}(F_{uv} + F_{vu}) - 2F_{uu} - 2F_{vv} \\
&= 2D_{uu}F^I_{vv} + 2D_{vv}F^I_{uu} - 4D_{uv}F^I_{vu} + 2\delta_{uv}(F_{uv} + F_{vu}) - 2F_{uu} - 2F_{vv} \\
&\quad - \sum_i \left(2(vv|ii) - (vi|iv)\right) + 4\sum_{pq} \left(d_{uupq}(vv|pq) + \left(d_{uqpu} + d_{uqup}\right)(vp|vq)\right) \\
&\quad + \sum_i \left(2(uv|ii) - (vi|iu)\right) - 4\sum_{pq} \left(d_{uvpq}(uv|pq) + \left(d_{uqpv} + d_{uqvp}\right)(up|vq)\right) \\
&\quad + \sum_i \left(2(vu|ii) - (vi|iu)\right) - 4\sum_{pq} \left(d_{vupq}(vu|pq) + \left(d_{vqpu} + d_{vqup}\right)(vp|uq)\right) \\
&\quad - \sum_i \left(2(uu|ii) - (ui|iu)\right) + 4\sum_{pq} \left(d_{vvpq}(uu|pq) + \left(d_{vqpv} + d_{vqvp}\right)(up|uq)\right) \\
&= 2D_{uu}F^I_{vv} + 2D_{vv}F^I_{uu} - 4D_{uv}F^I_{vu} + 2\delta_{uv}(F_{uv} + F_{vu}) - 2F_{uu} - 2F_{vv} \\
&\quad + 4\sum_{xy} \Big(d_{uuxy}(vv|xy) + \left(d_{uyxu} + d_{uyux}\right)(vx|vy) - d_{uvxy}(uv|xy) \\
&\quad - \left(d_{uyxv} + d_{uyvx}\right)(ux|vy) - d_{vuxy}(vu|xy) - \left(d_{vyxu} + d_{vyux}\right)(vx|uy) \\
&\quad + d_{vvxy}(uu|xy) + \left(d_{vyxv} + d_{vyvx}\right)(ux|uy)\Big)
\end{aligned}
\tag{7}
$$

# Fe(II)tpp Model System

Table S1: MBE-CASSCF energy for the lowest triplet and quintet states and corresponding energy gap of the Fe(II)tpp system for different screening parameters in a (22,22) active space with (6,6) and (8,8) reference spaces for the triplet and quintet states, respectively.

| Screening | Triplet Energy (in au) | Quintet Energy (in au) | Energy Gap (in kcal/mol) |
|---|---|---|---|
| medium | −2245.156547 | −2245.201957 | 28.50 |
| tight | −2245.156991 | −2245.202046 | 28.27 |
| very tight | −2245.157095 | −2245.202014 | 28.19 |
| 6 / 100% | −2245.156933 | −2245.201829 | 28.17 |

Table S2: MBE-CASSCF energy for the lowest triplet of the Fe(II)tpp system for different reference space sizes in a CAS(30,30) active space. The MBE was terminated after order 6.

| Reference Space | (6,6) | (8,8) |
|---|---|---|
| Triplet Energy (in au) | −2245.265808 | −2245.265273 |

Table S3: MBE-CASSCF energy for the lowest triplet and quintet states and corresponding energy gap of the Fe(II)tpp system for different active spaces and screening parameters. The triplet and quintet states used (6,6) and (8,8) reference spaces, respectively.

| CAS | Triplet Energy (in au) | Quintet Energy (in au) | Energy Gap (in kcal/mol) |
|---|---|---|---|
| HF | −2244.986964 | −2245.043905 | 35.73 |
| (22,22) | −2245.156933 | −2245.201829 | 28.17 |
| (30,30) | −2245.265808 | −2245.292189 | 16.55 |
| (40,40) | −2245.398154 | −2245.411361 | 8.29 |
| (50,50) | −2245.558638 | −2245.580548 | 13.75 |

# References

(S1) Siegbahn, P. E. M.; Almlöf, J.; Heiberg, A.; Roos, B. O. The complete active space SCF (CASSCF) method in a Newton–Raphson formulation with application to the HNO molecule. *J. Chem. Phys.* **1981**, *74*, 2384–2396.
